# Supplementary material for: Compressive Spectrum Sensing via Spectral Multiplexing in Rydberg Atomic Receiver
Source: arXiv:2607.02001 source file (2026-07-02)
Supplement: Supplementary file 2 [file SMref.tex]

\documentclass{article}
\begin{document}
\nocite{*}  % 引用所有文献
\bibliography{SM/SMref}  % 指定.bib文件名
\bibliographystyle{plain}  % 指定参考文献样式
\end{document}
